# Supplementary material for: Corps: A Core Calculus of Hierarchical Choreographic Programming
Source: arXiv:2406.01456 source file (2024-06-03)
Supplement: Supplementary file 1 [file appendices.tex]

% include appendices, similar to sections.tex

%%% Local Variables:
%%% mode: latex
%%% TeX-master: "conference"
%%% End:
